# Supplementary material for: Designing a boron nitride polyethylene composite for shielding neutrons
Source: arXiv:2211.09222 ancillary file (2023-10-04)
Supplement: Supplementary file 1 [file hBN_HDPE_Simulations_Supplemental.pdf]

## Supplemental Material

### Designing a boron nitride polyethylene composite for shielding neutrons

A. D. Vira,<sup>1</sup> E. Mone,<sup>1</sup> E. Ryan,<sup>2</sup> P. Connolly,<sup>3</sup> K. Smith,<sup>4</sup> C. Roecker,<sup>4</sup> K. Mesick,<sup>4</sup>

T. M. Orlando,<sup>5</sup> Z. Jiang,<sup>1</sup> and P. N. First<sup>1</sup>

<sup>1</sup>*School of Physics, Georgia Institute of Technology, Atlanta, GA 30332, USA*

<sup>2</sup>*School of Materials Science and Engineering, Georgia Institute of Technology, Atlanta, GA 30332, USA*

<sup>3</sup>*George W. Woodruff School of Mechanical Engineering, Georgia Institute of Technology, Atlanta, GA 30332, USA*

<sup>4</sup>*Space Science and Applications (ISR-1), Los Alamos National Laboratory, Los Alamos, NM 87545, USA*

<sup>5</sup>*School of Chemistry and Biochemistry, Georgia Institute of Technology, Atlanta, GA 30332, USA*

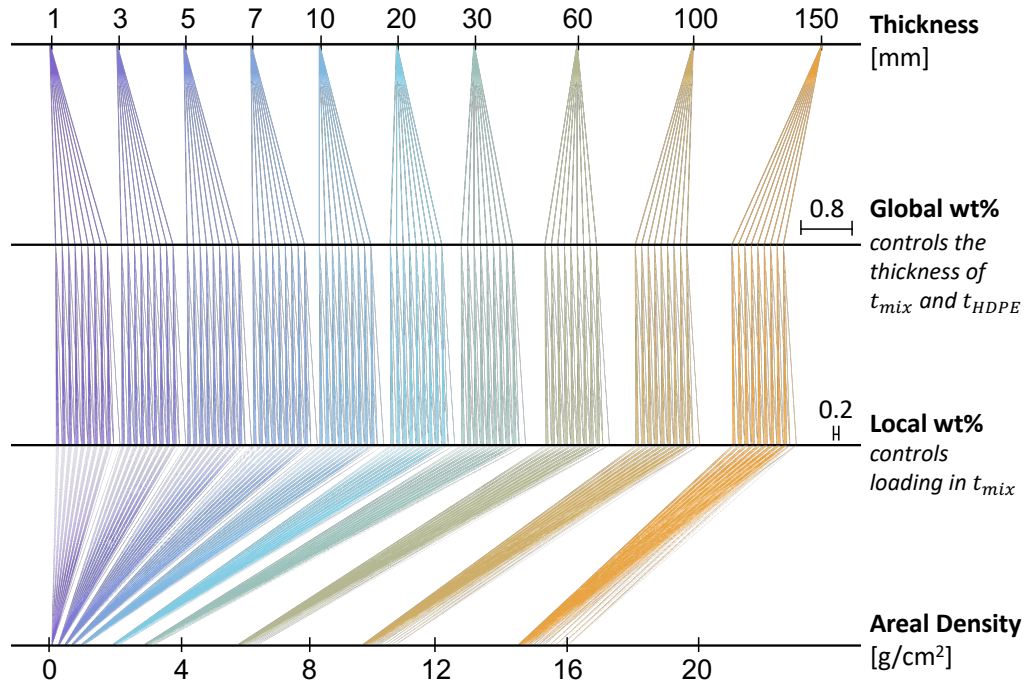

FIG. S1. Flowchart that shows how the thickness ( $t$ ), global weight percentage ( $\omega_{global}$ ), and local weight percentage ( $\omega_{local}$ ) are connected to the total areal density. Each composite with a unique thickness, ranging from 1 mm to 150 mm, is mapped to a unique  $\omega_{global}$ , ranging from 5 wt% to 95 wt%. Each unique  $\omega_{global}$  for each thickness is mapped to a unique  $\omega_{local}$ , ranging from 1 wt% to 20 wt%. The  $t$ ,  $\omega_{global}$ , and  $\omega_{local}$  are all used to calculate the areal densities. For cases where  $\omega_{global} \cdot \omega_{local}$  is equal to the same number for the same thicknesses but different combinations of  $\omega_{global}$  and  $\omega_{local}$ , the areal density is the same for those configurations. Otherwise, each combination of  $t$ ,  $\omega_{global}$ , and  $\omega_{local}$  is mapped to a unique areal density.

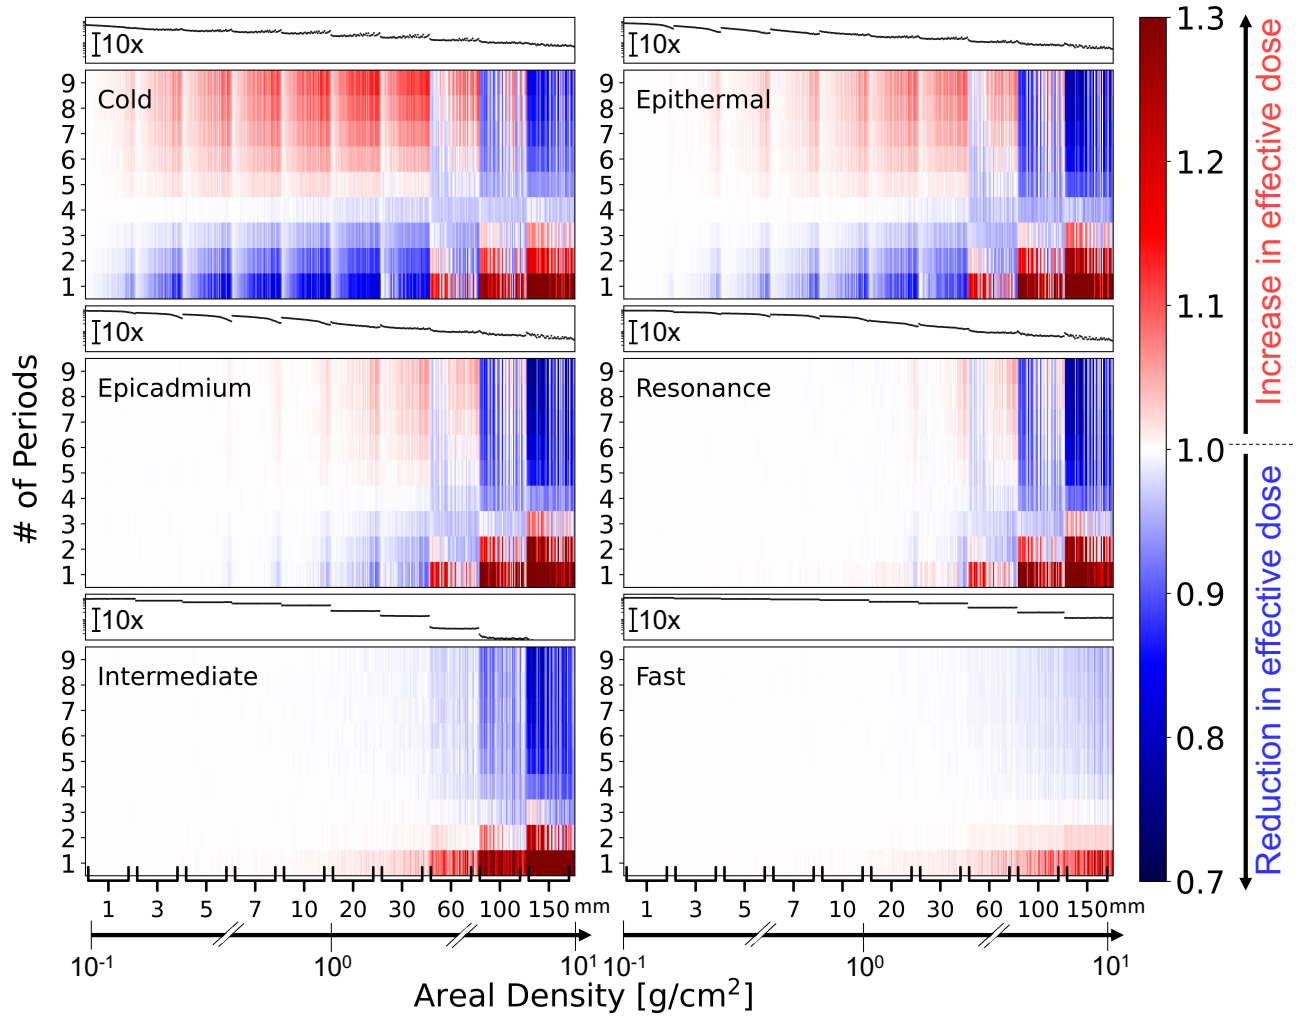

FIG. S2. Number of periods as a function of thickness/areal density, plotted on a nonlinear x-axis scale, for each energy range as labeled in each panel. Here, we bin all the manufacturable data and take the average effective dose for multiple points falling into the same bin. Each column is normalized to the average effective dose of the column, as shown in the lineplot above each 2D map (shown in color). The colorbar shows an increase, compared to the average effective dose in each column, in the effective dose in red and a reduction in the effective dose in blue. By dividing by the average effective dose of each column, one can easily tell if the trilayer or multilayer configuration is more optimal for that specific thickness and weight percentage. For each energy range (except for fast neutrons), the transition from trilayer to multilayer is evident. The transition seems to occur around a similar areal density.

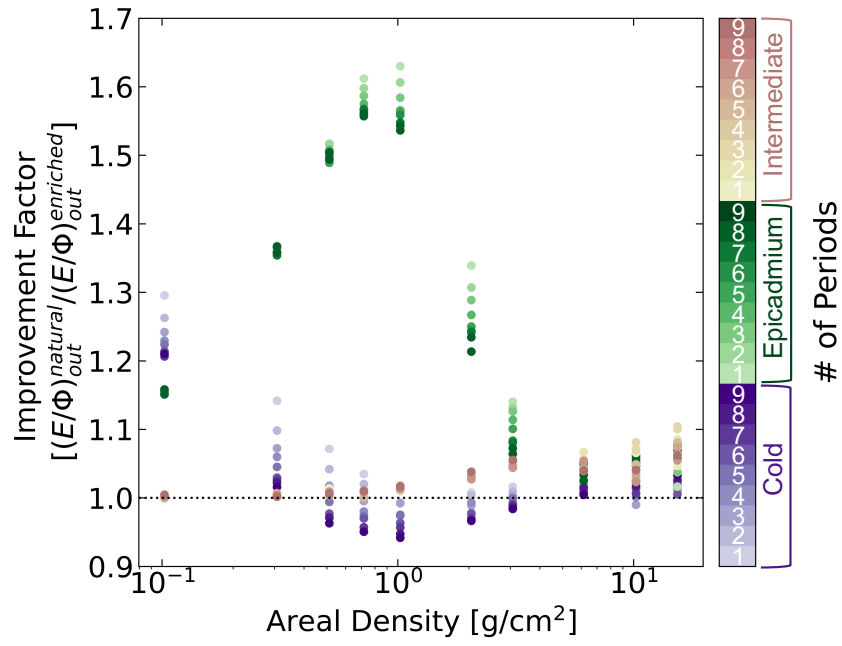

FIG. S3. Improvement factor  $[(E/\Phi)_{out}^{natural}/(E/\Phi)_{out}^{enriched}]$  as a function of areal density for three energy ranges (cold in shades of purple, epicadmium in shades of green, and intermediate in shades of brown). The variation in each shade corresponds to a different number of periods within the internal structure. The larger the improvement factor is the more beneficial it is to include  $^{10}\text{B}$  enriched hBN. Improvement factors around one means that the same shielding efficiency can be achieved with  $\text{h}^{Na}\text{BN}$ . For both cold and intermediate neutrons, there is not much improvement in using  $^{10}\text{B}$  enriched hBN. The same is true for fast neutrons (not shown). However, for epicadmium neutrons, there is an improvement up to 1.6 when using  $\text{h}^{10}\text{BN}$ .
